# Supplementary material for: Symmetry and Classification of Multipartite Entangled States
Source: arXiv:2204.13441 source file (2022-04-28)
Supplement: Supplementary file 1 [file supplemental_material.pdf]

# Supplemental Material: Entanglement classification via Roots of Polynomial Invariants

## SECTION 1. PROOF OF THEOREM 1

We present a proof for Theorem 1. Any  $n + 1$  partite qubit state  $|\psi\rangle \in \mathcal{H}_2^{\otimes(n+1)}$  might be written as

$$|\psi\rangle = |0\rangle |\psi_0\rangle + |1\rangle |\psi_1\rangle. \quad (\text{S1})$$

Such a form provides the canonical decomposition of the reduced density matrix  $\rho = |\psi_0\rangle \langle \psi_0| + |\psi_1\rangle \langle \psi_1|$  over the non-normalized states  $|\psi_0\rangle, |\psi_1\rangle \in \mathcal{H}_2^{\otimes N}$ , obtained by tracing out the first qubit. Consider now a reversible operator  $\mathcal{O} = \begin{pmatrix} a & b \\ c & d \end{pmatrix} \in \text{SL}(2, \mathbb{C})$  acting on the first qubit. Under the action of this operator, the state  $|\psi\rangle$  is transformed into

$$|\psi'\rangle := \mathcal{O} |\psi\rangle = |0\rangle (a |\psi_0\rangle + b |\psi_1\rangle) + |1\rangle (c |\psi_0\rangle + d |\psi_1\rangle) = |0\rangle |\psi'_0\rangle + |1\rangle |\psi'_1\rangle, \quad (\text{S2})$$

where

$$|\psi'_0\rangle := a |\psi_0\rangle + b |\psi_1\rangle, \quad (\text{S3})$$

$$|\psi'_1\rangle := c |\psi_0\rangle + d |\psi_1\rangle. \quad (\text{S4})$$

Consider now any superposition of states  $|\psi'_0\rangle$  and  $|\psi'_1\rangle$ . Observe that

$$\begin{aligned} |\psi'_z\rangle &:= z |\psi'_0\rangle + |\psi'_1\rangle = z(a |\psi_0\rangle + b |\psi_1\rangle) + c |\psi_0\rangle + d |\psi_1\rangle \\ &= (az + b) |\psi_0\rangle + (cz + d) |\psi_1\rangle \\ &\propto \frac{az + b}{cz + d} |\psi_0\rangle + |\psi_1\rangle, \end{aligned}$$

where the complex number  $cz + d$  was factored out in order for the transformation to map states from the extended plane representation to the extended plane representation. In other words, we have

$$\mathcal{O} |\psi_z\rangle = |\psi_{z'}\rangle, \quad z' = \frac{az + b}{cz + d}, \quad (\text{S5})$$

i.e. the operator  $\mathcal{O}$  transforms states in the extended plane representation by applying a Möbius transformation on the index  $z$ . Suppose now that  $\zeta_i$  is a zero of a  $h$ -degree polynomial function  $E$ , i.e.  $E(\zeta_i |\psi_0\rangle + |\psi_1\rangle) = 0$ . Acting on the first qubit with  $\mathcal{O}$ , the density matrix after tracing out the first qubit becomes  $|\psi'_0\rangle \langle \psi'_0| + |\psi'_1\rangle \langle \psi'_1|$ , so the entanglement measure  $E$  will be zero for some new roots  $\zeta'_i$ , such that  $E(\zeta'_i |\psi'_0\rangle + |\psi'_1\rangle) = 0$ . Using Eqs. (S3)-(S4), the later equation can be transformed into

$$E \left( (c\zeta'_i + d) \left( \frac{a\zeta'_i + b}{c\zeta'_i + d} |\psi_0\rangle + |\psi_1\rangle \right) \right) = 0 \quad (\text{S6})$$

where the factor  $(c\zeta'_i + d)$  is irrelevant since any root multiplied by it will still be a valid root. Comparing with the equation for the roots before the action of  $\mathcal{O}$ , we reach the conclusion that the roots transform according to the inverse Möbius transformation as

$$\zeta'_i = \frac{d\zeta_i - b}{-c\zeta_i + a}, \quad (\text{S7})$$

under the action of the operator  $\mathcal{O}$ . As a consequence, the roots of the zero-polytope transform with respect to the inverse Möbius transformation associated to the operator  $\mathcal{O} = \begin{pmatrix} a & b \\ c & d \end{pmatrix}$ . Analyze now the case when  $\mathcal{O}$  is a unitary operator  $\mathcal{O} = \mathcal{U}$ . Since any unitary operator  $\mathcal{U}$  can be represented as a rotation  $\mathcal{R} = \begin{pmatrix} \cos\alpha & \sin\alpha e^{i\phi} \\ -\sin\alpha e^{-i\phi} & \cos\alpha \end{pmatrix}$  (up to an irrelevant global phase), it will simply rotate the Bloch ball, together with the zero-polytope.

Consider now multilocal operators  $\mathcal{O}_{\vec{n}} = \mathcal{O}_1 \otimes \dots \otimes \mathcal{O}_n$  acting on the remaining qubits of the state  $|\psi\rangle$  from Eq. (S1). The state  $|\psi\rangle$  will transform accordingly as

$$|\psi'\rangle := \mathcal{O}_{\vec{n}} |\psi\rangle = |0\rangle \underbrace{\mathcal{O}_{\vec{n}} |\psi_0\rangle}_{:=|\psi'_0\rangle} + |1\rangle \underbrace{\mathcal{O}_{\vec{n}} |\psi_1\rangle}_{:=|\psi'_1\rangle}. \quad (\text{S8})$$

After the action of  $\mathcal{O}_{\vec{n}}$ , a state in the extended plane representation will have a value of entanglement measure  $E$  equal to

$$E\left(z|\psi'_0\rangle + |\psi'_1\rangle\right) = E\left(\mathcal{O}_{\vec{n}}(z|\psi_0\rangle + |\psi_1\rangle)\right).$$

However, since  $E$  is  $\text{SL}(2, \mathbb{C})^{\otimes n}$  invariant, we have that  $E(z|\psi_0\rangle + |\psi_1\rangle) = 0$  iff  $E(z|\psi'_0\rangle + |\psi'_1\rangle) = 0$ , and so the roots of both polynomial equations are the same. As a consequence, the roots of the the zero-polytope will remain unchanged under the action of  $\mathcal{O}_{\vec{n}}$ . This concludes the proof of Theorem 1.

## SECTION 2. NORMAL FORM

Consider the set of four symmetrically related points  $\Phi = \{z, \frac{1}{z}, -z, -\frac{1}{z}\}$ . It is very convinient to associate with them the cuboid spanned by eight points:

$$\Phi \cup \bar{\Phi} = \left\{z, \frac{1}{z}, -z, -\frac{1}{z}, \bar{z}, \frac{1}{\bar{z}}, -\bar{z}, -\frac{1}{\bar{z}}\right\},$$

as it is presented on Figure S1. Observe, that all six faces of the cuboid are parallel to one of the planes:  $XZ, XY$ , or  $YZ$ . In fact, this property is equivalent to the initial assumption that the set of points  $\Phi$  is in normal form. Clearly, all rotations of the Bloch ball preserve the form of the cuboid. Nevertheless, only a special subgroup of all rotations preserve faces of the cuboid being parallel to  $XZ, XY$ , or  $YZ$ . This special subgroup  $\mathcal{G}_{24}$  contains 24 elements spanned by three rotations of  $\pi/2$  around  $X, Y$ , and  $Z$  axis, given by:

$$\mathbf{R}_x(\pi/2) = \begin{pmatrix} \cos \pi/4 & -i \sin \pi/4 \\ -i \sin \pi/4 & \cos \pi/4 \end{pmatrix} = \frac{1}{\sqrt{2}} \begin{pmatrix} 1 & -i \\ -i & 1 \end{pmatrix}, \quad (\text{S9})$$

$$\mathbf{R}_y(\pi/2) = \begin{pmatrix} \cos \pi/4 & -\sin \pi/4 \\ \sin \pi/4 & \cos \pi/4 \end{pmatrix} = \frac{1}{\sqrt{2}} \begin{pmatrix} 1 & -1 \\ 1 & 1 \end{pmatrix}, \quad (\text{S10})$$

$$\mathbf{R}_z(\pi/2) = \begin{pmatrix} e^{-i\pi/4} & 0 \\ 0 & e^{i\pi/4} \end{pmatrix} = \frac{1}{\sqrt{2}} \begin{pmatrix} 1-i & 0 \\ 0 & 1+i \end{pmatrix} \quad (\text{S11})$$

In fact, this is a group of rotations preserving the regular cube (the group of orientable cube symmetries). Clearly, all rotations in the  $\mathcal{G}_{24}$  group preserve the normal-form structure of  $\Phi$ . On the other hand, the normal form is uniquely determined up to 24 rotations in the  $\mathcal{G}_{24}$  group.

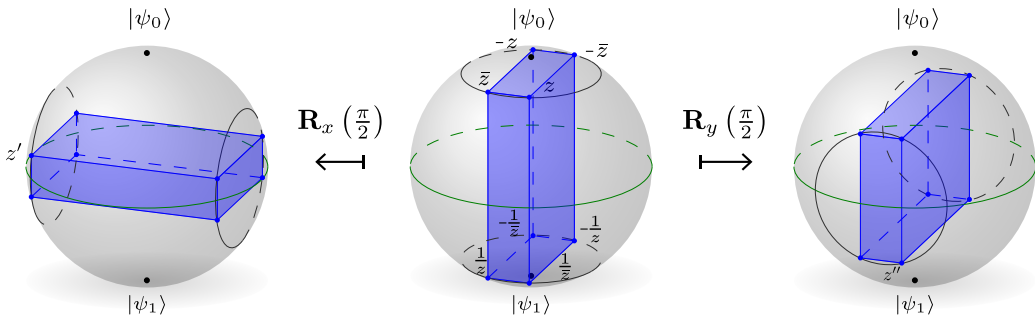

**Figure S1.** A normal system of roots  $z, 1/z, -z, -1/z$  together with the conjugate points  $\bar{z}, 1/\bar{z}, -\bar{z}, -1/\bar{z}$  span the cuboid whose faces are parallel to the  $XZ, XY$  and  $YZ$  planes. There are 24 rotations of the Bloch sphere which preserve this property, composing the elements of the group  $\mathcal{G}_{24}$ . Two of them, namely the rotation by a  $\pi/2$  angle around  $X$  and  $Y$  axes are presented. The system of roots transforms according to Eqs. S9-S11, giving  $z \mapsto z' := \frac{z-i}{-iz+1}$  and  $z \mapsto z'' := \frac{z-1}{z+1}$  for the two rotations.

**Proposition 1.** Each non-degenerated four points  $z_1, z_2, z_3, z_4$  on the Bloch sphere can be transformed onto the normal form  $z, \frac{1}{z}, -z, -\frac{1}{z}$  via a Möbius transformation  $T$ . The latter is uniquely defined up to 24 rotations in the group  $\mathcal{G}_{24}$ .

*Proof.* For each complex number  $\lambda$  there exists another complex number  $z$ , such that the cross-ratio of the four points is equal to  $\lambda$ , i.e.

$$\left(z, \frac{1}{z}; -z, -\frac{1}{z}\right) = \lambda. \quad (\text{S12})$$

Indeed, the cross-ratio on the left side equals  $4z^2/(1+z^2)^2$ , and the equation  $4z^2/(1+z^2)^2 = \lambda$  has exactly four solutions

$$z_0 = \frac{4 - 2\lambda + \sqrt{1 - \lambda}}{2\lambda}, \frac{1}{z_0}, -z_0, -\frac{1}{z_0}. \quad (\text{S13})$$

Therefore, for a given value  $\lambda$  there exists a unique  $\lambda$ -normal system, such that the cross-ratio of its vertices is given by  $(z_0, \frac{1}{z_0}; -z_0, -\frac{1}{z_0}) = \lambda$ . Replacing the vertex  $z_0$  by any other vertex  $z_0, 1/z_0, -z_0$ , or  $-1/z_0$  does not change the value of the cross-ratio  $(z_0, \frac{1}{z_0}; -z_0, -\frac{1}{z_0}) = \lambda$ . Note that there exists a unique Möbius transformation  $T$  which maps  $z_1, z_2, z_3$  onto  $z_0, 1/z_0, -z_0$ , with the remaining  $z_4$  mapped onto  $-1/z_0$ . Observe as well that the value of  $z_0$  is unique up to its inverse, opposite and opposite inverse elements, according to Eq. (S13), with the corresponding Möbius transformations associated to the matrices  $T, \sigma_x T, \sigma_y T$  and  $\sigma_z T$ . Each of those transformations maps the set of points  $\{z_1, z_2, z_3, z_4\}$  onto the same set of points  $\{z_0, 1/z_0, -z_0, -1/z_0\}$ , although the exact bijection between those two sets of roots is different for each transformation.

Depending on the order of four points  $\{z_1, z_2, z_3, z_4\}$ , the corresponding cross-ratio takes six values:  $\lambda, \frac{1}{\lambda}, 1 - \lambda, \frac{1}{1-\lambda}, \frac{\lambda-1}{\lambda}$  and  $\frac{\lambda}{\lambda-1}$ . For each of these, there is a corresponding set of solutions of the form  $\{z_0, 1/z_0, -z_0, -1/z_0\}$  via Eq. (S13) with four related Möbius transformations. Therefore, there are in total 24 Möbius transformations that map any four non-degenerated points onto a normal system, each of them related by an element of the group  $\mathcal{G}_{24}$  which has exactly 24 elements.  $\square$

### SECTION 3. PROOF OF PROPOSITION 1

Consider the state  $|G_{abcd}\rangle$  and its decomposition with respect to the first subsystem  $|G_{abcd}\rangle = |0\rangle|\psi_0\rangle + |1\rangle|\psi_1\rangle$ , where

$$\begin{aligned} |\psi_0\rangle &= \frac{a+d}{2}|000\rangle + \frac{a-d}{2}|011\rangle + \frac{b+c}{2}|101\rangle + \frac{b-c}{2}|110\rangle, \\ |\psi_1\rangle &= \frac{a+d}{2}|111\rangle + \frac{a-d}{2}|100\rangle + \frac{b+c}{2}|010\rangle + \frac{b-c}{2}|001\rangle. \end{aligned}$$

Suppose that  $\tau^{(3)}(\zeta|\psi_0\rangle + |\psi_1\rangle) = 0$ . Since  $\tau^{(3)}$  is a  $\text{SL}(2, \mathbb{C})^{\otimes 3}$  invariant, for any local operators  $\mathcal{O}_1, \mathcal{O}_2, \mathcal{O}_3$  we have

$$\tau^{(3)}\left((\mathcal{O}_1 \otimes \mathcal{O}_2 \otimes \mathcal{O}_3)(\zeta|\psi_0\rangle + |\psi_1\rangle)\right) = 0.$$

Observe that

$$\begin{aligned} |\psi_0\rangle &= (\sigma_x \otimes \sigma_x \otimes \sigma_x) |\psi_1\rangle, \\ |\psi_1\rangle &= (\sigma_x \otimes \sigma_x \otimes \sigma_x) |\psi_0\rangle, \end{aligned}$$

where  $\sigma_x, \sigma_y, \sigma_z$  are Pauli matrices. Therefore by taking all local operators  $\mathcal{O}_1, \mathcal{O}_2, \mathcal{O}_3$  equal to  $\sigma_x$ , we may conclude that

$$0 = \tau^{(3)}\left((\sigma_x \otimes \sigma_x \otimes \sigma_x)(\zeta|\psi_0\rangle + |\psi_1\rangle)\right) = \zeta|\psi_1\rangle + |\psi_0\rangle \propto \frac{1}{\zeta}|\psi_0\rangle + |\psi_1\rangle, \quad (\text{S14})$$

hence  $1/\zeta$  is another root of  $\tau^{(3)}$ . Similarly, by considering  $(\sigma_y \otimes \sigma_y \otimes \sigma_y)$  and  $(\sigma_z \otimes \sigma_z \otimes \sigma_z)$ , one may find another two roots  $-\zeta, -1/\zeta$  of  $\tau^{(3)}$ . This shows that the roots of  $\tau^{(3)}$  evaluated on any state from the  $G_{abcd}$  family are symmetrical with respect to rotations around  $X, Y, Z$  axes by the angle  $\pi$ . Writting  $\tau^{(3)}(z|\psi_0\rangle + |\psi_1\rangle) = 0$  explicitly, we obtain the equation

$$\tau^{(3)}(z|\psi_0\rangle + |\psi_1\rangle) = Az^4 - 2(2B + A)z^2 + A = 0, \quad (\text{S15})$$

where  $A = (b^2 - c^2)(a^2 - d^2)$  and  $B = (c^2 - d^2)(a^2 - b^2)$ . The above equation is non-degenerated iff  $A, B, A + 2B \neq 0$ , which happens iff  $a^2 \neq b^2 \neq c^2 \neq d^2$  are pairwise different.

**Lemma 1.** Any local operator  $\mathcal{O} = \mathcal{O}_1 \otimes \mathcal{O}_2 \otimes \mathcal{O}_3 \otimes \mathcal{O}_4 \in \text{SL}(2, \mathbb{C})^{\otimes 4}$  which transforms states  $|G_{a'b'c'd'}\rangle \propto \mathcal{O} |G_{abcd}\rangle$  with  $a^2 \neq b^2 \neq c^2 \neq d^2$ , is of the form  $\mathcal{O}_i \in \mathcal{G}_{24}$ .

*Proof.* A local operator  $\mathcal{O}_1$  acting on the first qubit and transforming the state  $|G_{abcd}\rangle$  onto  $|G_{a'b'c'd'}\rangle$ , also transforms their systems of roots denoted as  $\Lambda$  and  $\Lambda'$ , respectively, via the action of the corresponding Möbius transformation. Note that both systems  $\Lambda$  and  $\Lambda'$  are in the normal form, therefore, according to Proposition 1, we have that  $\mathcal{O}_i \in \mathcal{G}_{24}$ . A similar analysis with respect to all other qubits shows that  $\mathcal{O}_2, \mathcal{O}_3, \mathcal{O}_4 \in \mathcal{G}_{24}$ .  $\square$

This way, searching for SLOCC-equivalence between the states  $|G_{abcd}\rangle$  and  $|G_{a'b'c'd'}\rangle$  becomes restricted to the search within the finite class of operators  $\mathcal{O} \in \mathcal{G}_{24}^{\otimes 4}$ . Since the group  $\mathcal{G}_{24}$  has only 24 elements, one may numerically verify that there are exactly  $8 \times 24 = 192$  states in the  $G_{abcd}$  family which are SLOCC-equivalent to  $|G_{abcd}\rangle$  by  $\mathcal{O} \in \mathcal{G}_{24}^{\otimes 4}$ . For example, the following operation

$$\mathbf{R}_x\left(\frac{\pi}{2}\right) \otimes \mathbf{R}_x\left(\frac{\pi}{2}\right) \otimes \mathbf{R}_x\left(\frac{\pi}{2}\right) \otimes \mathbf{R}_x\left(\frac{\pi}{2}\right) \quad (\text{S16})$$

transforms state  $|G_{abcd}\rangle$  into  $|G_{-b,-a,c,d}\rangle$ . This might be simply written as a transformation of a tuples of indices: the tuple  $(a, b, c, d)$  is transformed into the tuple  $(-b, -a, c, d)$ . Similarly, the operators showed on the following right hand sides provide the corresponding transformations of the tuple  $(a, b, c, d)$  on the left side:

$$\begin{aligned} \mathbf{R}_y\left(\frac{\pi}{2}\right) \otimes \mathbf{R}_y\left(\frac{\pi}{2}\right) \otimes \mathbf{R}_y\left(\frac{\pi}{2}\right) \otimes \mathbf{R}_y\left(\frac{\pi}{2}\right) &\longleftrightarrow (a, \textcolor{blue}{d}, c, \textcolor{blue}{b}), \\ \mathbf{R}_z\left(\frac{\pi}{2}\right) \otimes \mathbf{R}_z\left(\frac{\pi}{2}\right) \otimes \mathbf{R}_z\left(\frac{\pi}{2}\right) \otimes \mathbf{R}_z\left(\frac{\pi}{2}\right) &\longleftrightarrow (-\textcolor{blue}{d}, b, c, -a), \\ \mathbf{R}_y(\pi) \otimes \mathbf{R}_y(\pi) \otimes \mathbf{1} \otimes \mathbf{1} &\longleftrightarrow (a, -\textcolor{blue}{b}, -\textcolor{blue}{c}, d), \\ \mathbf{R}_x(\pi) \otimes \mathbf{R}_x(\pi) \otimes \mathbf{1} \otimes \mathbf{1} &\longleftrightarrow (a, b, -\textcolor{blue}{c}, -\textcolor{blue}{d}), \\ \mathbf{R}_y(\pi) \otimes \mathbf{1} \otimes \mathbf{R}_y(\pi) \otimes \mathbf{1} &\longleftrightarrow (\textcolor{blue}{d}, c, b, a), \\ \mathbf{R}_x(\pi) \otimes \mathbf{1} \otimes \mathbf{R}_x(\pi) \otimes \mathbf{1} &\longleftrightarrow (b, a, \textcolor{blue}{d}, c). \end{aligned}$$

Additionally, the tuples  $(a, b, c, d)$  and  $(-a, -b, -c, -d)$  represent the same state. Note that any composition of the above operations also provides SLOCC equivalences between  $|G_{abcd}\rangle$  states. The eight aforementioned transformations of tuples generate all permutations of the  $a, b, c, d$  indices, together with the change of a sign of any two or all four indices. There are exactly 24 permutations and for each permutation the signs can be matched in exactly  $1 + \binom{4}{2} + 1 = 8$  ways. This gives in total 192 tuples representing SLOCC equivalent states, which perfectly matches the numerical result.

Finally, another trivial manipulation with indices  $a, b, c, d$  comes from multiplying by a global phase, which is an irrelevant operation due the fact that quantum states are elements of a projective space. This operation transforms the indices as

$$(e^{i\theta}a, e^{i\theta}b, e^{i\theta}c, e^{i\theta}d) \sim (a, b, c, d),$$

resulting in the same quantum state for any real number  $\theta \in [0, 2\pi)$ . In particular, for  $\theta = \pi$ , we observe that system of opposite indices determines the same state as the initial one, i.e.  $(-a, -b, -c, -d) \sim (a, b, c, d)$ .
